# Supplementary material for: Rethinking Sensors Modeling: Hierarchical Information Enhanced Traffic Forecasting
Source: arXiv:2309.11284 source file (2023-09-20)
Supplement: Supplementary file 1 [file 8_Appendix.tex]

\section{Appendix}

\begin{algorithm}%[t]
	\caption{\label{alg:algorithm1} 
    The pipeline of proposed \name. 
	% Optimizing pipeline of \name.
 % ,$\boldsymbol{{H}}_r^*$ and $\boldsymbol{{H}}_g^*$.
	}
	\raggedright
	{\bf Input}:  Processed data $\boldsymbol{H}_o$ with the shape $(B, T, N_o,D)$ , the mapping matrix $\boldsymbol{M}_{or}$ via solving BCC and the adjacency matrix of the original graph $\boldsymbol{A}_{o}$  and regional graph $\boldsymbol{A}_{r}$ via \eqref{eq:mapAor}.
 \\
	{\bf Output}: The optimized parameters $\theta^*$ of \name\\ %The prediction value $\boldsymbol{\hat{X}}_o$ with the shape $(B, T, N_o,D)$ \\%The enhanced representation of the original graph $\boldsymbol{{H}}_o^*$\\
    % \textbf{Stage 1. Pretrain the spatio-temporal transformer.}\\
	\begin{algorithmic} [1]
        % \State \textbf{Stage I. Pretrain the spatio-temporal transformer.}
        % \State //{Initialization}
        \State Initialize the trainable mapping matrix $\boldsymbol{M}_{rg}$ and other network parameters $\theta$
        % \State Init()
        \State epoch $\leftarrow$ 0
        \While{epoch < MaxEpoch}
        \State Generate $\boldsymbol{A}_{g}$ via \eqref{eq:mapArg}
        \For{$l$ in $\mathcal{L}$ layers}
        % \State if $l$==0: $X_o = H_o$ else: $X_o = H_o^*\ from\ (l-1)th\ layer$ 
        \State $\boldsymbol{H}_o$ $\leftarrow$ TCN($\boldsymbol{X}$) \eqref{eq:TCN}
        \State Add Skip\_connection($\boldsymbol{H}_o$)
        \State //{\gcnname}
        \State Generate $\boldsymbol{H}_{r} $ via \eqref{eq:mapHor} and $\boldsymbol{H}_{g} $ via \eqref{eq:mapHrg}
        \State $\boldsymbol{H}_o^* \leftarrow$ enhance process via \eqref{eq:gr}, \eqref{eq:ro}
        \State $\boldsymbol{H}_r^*$,$\boldsymbol{H}_g^* \leftarrow$
        update process via  \eqref{eq:or},\eqref{eq:rg}
        \EndFor
        \State //{Prediction}
        \State $\boldsymbol{\hat{X}}_o$ = OutputLayer(Skip($\boldsymbol{H}_o^*$))
        % \State //{Calculate loss}
        \State //{Prediction loss} 
        \State $\mathcal{L}_{pre}$ = MAE($\boldsymbol{\hat{X}}_o$ - $\boldsymbol{X}_o$ ) via \eqref{eq:fineLoss}
        % \State //{Reconstrcution loss}
        \State //Get the adjacency matrix of original and regional graph 
        \State $\boldsymbol{\hat{A}}_{o} \leftarrow$ \eqref{eq:reconstruct0} and $\boldsymbol{\hat{A}}_{r} \leftarrow$ \eqref{eq:reconstruct1}
        % \State //Construct the adjacency matrix of regional graph
        % \State $\boldsymbol{\hat{A}}_{r} \leftarrow$ \eqref{eq:reconstruct1}
        % \State //Compute the reconstruction loss $\mathcal{L}_{rec_{ro}}$ 
        \State $\mathcal{L}_{rec_{ro}} \leftarrow \mathcal{L}_{rec}(\boldsymbol{\hat{A}}_{o},\boldsymbol{{A}}_{o})$ via  \eqref{eq:BCELossro}
        % \State //Compute the reconstruction loss $\mathcal{L}_{rec_{gr}}$ 
        \State $\mathcal{L}_{rec_{gr}} \leftarrow \mathcal{L}_{rec}(\boldsymbol{\hat{A}}_{r},\boldsymbol{{A}}_{r})$via \eqref{eq:BCELossgr}
        % \State //{Orthognoal loss}
        \State $\mathcal{L}_{ort} \leftarrow$ the Orthogonal loss computed via  \eqref{eq:orthLoss}
        \State $\theta \leftarrow$ Optimize the objective function $\mathcal{L} \eqref{eq:objection}$ %\mathcal{L}_{pre} + \mathcal{L}_{rec_{ro}} + \mathcal{L}_{rec_{gr}} + \mathcal{L}_{ort} $ \eqref{eq:objection}
        \State epoch++
        \EndWhile
        \State
	    {\bf Return}:$\theta^*$%$\boldsymbol{{H}}_o^*$%,$\boldsymbol{{H}}_r^*$ and $\boldsymbol{{H}}_g^*$
	\end{algorithmic}
\end{algorithm}
